# Supplementary material for: SCTc-TE: A Comprehensive Formulation and Benchmark for Temporal Event Forecasting
Source: arXiv:2312.01052 source file (2024-04-03)
Supplement: Supplementary file 1 [file 8_appendix.tex]

\appendix
\section{Appendix}~\label{sec:appendix}
\subsection{SCTc-TE Construction Pipeline}~\label{app:subsec:dataset_construction}
We present more details of the SCTc-TE construction pipeline, including the news article filtering in the data pre-processing stage, the complex event identification stage, and the event extraction stage. Finally, we present the evaluation settings of our datasets.
\subsubsection{News Article Filtering}
We first keep the atomic events of which the locations are EG, IR, and IS. Then we download the articles with valid URLs, excluding those news articles of which the URLs are broken or unaccessible. Moreover, we sort the news agencies (identified by the domain names of the URLs) based on the number of published news articles in descending order, and keep the top 69 news agencies that takes over 40\% of all the news articles in GDELT dataset. This step can largely reduce the amount of low-quality news articles, which are with poor writings or even fake news. After these filtering, we keep 586,691 news articles. 

\begin{table*}[t]
\caption{The detailed dataset statistics of MidEast-TE.}
\vspace{-0.1in}
\label{tab:clustering_stats}
\centering
\setlength{\tabcolsep}{1mm}{
    \resizebox{0.99\textwidth}{!}{
        \begin{tabular}{l c c c c ccc ccc}
        \toprule
        \multirow{2.4}{*}{$\lambda$} & \multirow{2.4}{*}{\shortstack{minimum \\ cluster size}} & \multirow{2.4}{*}{\#clusters} & \multirow{2.4}{*}{\%outlier doc} & \multirow{2.4}{*}{\shortstack{\%outlier \\ atomic events}} & \multicolumn{3}{c}{\#atomic events} & \multicolumn{3}{c}{\#time span (days)} \\
        \cmidrule(lr){6-8} \cmidrule(lr){9-11} & & & & & max & min & avr & max & min & avr \\
        \midrule
        0 & 10 & 1,653 & 53.93 & 54.60 & 3,257  & 10 & 145.82 & 2,583 & 2  & 1682.16 \\
        1 & 5  & 9,126 & 46.13 & 46.82 & 1,318  & 5  & 30.96  & 1,018 & 1  & 22.74   \\
        \underline{1} & \underline{10} & \underline{3,750} & \underline{52.52} & \underline{52.52} & \underline{4,541}  & \underline{10} & \underline{67.27}  & \underline{2,568} & \underline{2}  & \underline{39.25}   \\
        1 & 30 & 973  & 60.19 & 59.33 & 10,342 & 34 & 222.08 & 2,568 & 2  & 85.53   \\
        1 & 50 & 525  & 63.18 & 62.31 & 10,268 & 55 & 381.38 & 2,567 & 11 & 114.18  \\
        \bottomrule
        \end{tabular}
    }
}
\vspace{-0.1in}
\end{table*}

We further remove the news articles that do not report any atomic events that are defined in the CAMEO ontology or only contain long-tailed actors (occur less than 10 times or appear in less than 10 news articles) based on the our own EE results (this will be introduced in the following Section~\ref{subsubsec:EE}). Finally, we keep 275,406 documents, which is about 47\% of all the news articles in the prior step. This step removes a large portion of news articles that are irrelevant to the CAMEO ontology or rarely occurring actors, thus resulting in that our datasets focus on the most salient and active actors and events in this region. Therefore, the remaining news articles in our datasets are characterized with high quality.

\subsubsection{Complex Event Identification}
For the document clustering, we use the RoBERTa model that is fine-tuned with SimCSE~\footnote{\url{https://github.com/princeton-nlp/SimCSE}} to extract the document embedding. We just concatenate the title and the whole document and take the first 512 token as input to extract the article embeddings. We use the default setting of 200 as the number of neighbors in UMAP. For HDBSCAN, we tune the hyper-parameter of \textit{minimum cluster size} from $\{5,10,30,50\}$. We tune the temporal feature weight $\lambda$ from $\{0,1\}$. The clustering results of various settings are shown in Table~\ref{tab:clustering_stats}. When $\lambda=0$, which means we do not consider the temporal feature and solely rely on the semantic features of the news articles for the clustering, the average time span of the cluster (CE) is extremely large as 1682 days (4.6 years). In contrast, by setting $\lambda=1$, the average time span of CEs is largely reduced, showing that incorporating the temporal feature into the clustering applies effective constraint for the temporal conciseness of CEs. To select the best parameter for \textit{minimum cluster size}, we empirically take 10, which will result in a reasonable scale for the average cluster size, \wrt both \#atomic events (67.27) and \#time span (39.25). It should be noted that there are about half of all the news articles being clustered as \textit{outliers}, which is reasonable for the density-based clustering method (HDBSCAN). This clustering method is rigorous when including an article to a specific cluster, assuring the compactness of the CEs.

After the clustering, there are a few clusters that are extremely large, for example, the max cluster has 4541 atomic events and spans 2568 days. We divide such super clusters into multiple smaller clusters. Specifically, we take a greedy strategy that we accumulate the articles and atomic events from the first timestamp of the super clusters; when either the number of articles reaches $h_a$ or the length of time span reaches $h_t$, we cutoff the super cluster and assign the accumulated atomic events into a new cluster. Then we repeat this process on the remaining part of the super cluster. Such iteration ends when the remaining part does not exceed either of the two threshold $h_a$ and $h_t$. For MidEast-TE, we empirically set $h_a=112$ and $h_t=78$, which are just twice of the average size of the original clusters. Then we remove the clusters that are shorter than two days or fewer than 10 atomic events. We split the clusters into training/validation/testing set according to the weighted centroid of the timestamp distribution. We further remove the atomic events in the validation and testing set whose entities and relations are new and have not appeared in the training set, thus preventing the cold-start problem during forecasting. We present the detailed statistics of MidEast-TE in Table~\ref{tab:detailed_stats_mideast}. We take the same pre-processing steps for the GDELT-TE dataset, the detailed statistics of which is shown in Table~\ref{tab:detailed_stats_gdelt}. It should be noted that the number of CEs in GDELT-TE has a small shift to MidEast-TE, even though they are based on the same document clustering results. This is because certain steps of the filtering are based on the extracted atomic events, which are different for the two datasets.

\begin{table*}[t]
\caption{The detailed statistics of MidEast-TE.}
\vspace{-0.1in}
\label{tab:detailed_stats_mideast}
\centering
\setlength{\tabcolsep}{1mm}{
    \resizebox{0.9\textwidth}{!}{
        \begin{tabular}{l c c c c c ccc ccc}
        \toprule
        \multirow{2.4}{*}{subset} & \multirow{2.4}{*}{\#docs} & \multirow{2.4}{*}{\shortstack{\#ttl atomic \\ events}} & \multirow{2.2}{*}{$|\mathcal{E}|$} & \multirow{2.4}{*}{$|\mathcal{R}|$} & \multirow{2.4}{*}{\#CEs} & \multicolumn{3}{c}{\#atomic events/CE} & \multicolumn{3}{c}{\#time span (days)} \\
        \cmidrule(lr){7-9} \cmidrule(lr){10-12} & & & & & & max & min & avr & max & min & avr \\
        \midrule
        train   & 90,252  & 160,953 & 2,641 & 218 & 3,452 & 112 & 10 & 46.63 & 78 & 2 & 30.11 \\
        val     & 13,532  & 25,401  & 1,281 & 176 & 492   & 112 & 10 & 51.53 & 78 & 2 & 34.33 \\ 
        test    & 12,333  & 22,440  & 1,183 & 177 & 453   & 112 & 10 & 49.54 & 78 & 2 & 34.92 \\
        outlier & 137,802 & 247,083 & 2,760 & 227 & -     & -   & -  & -     & -  & - & -     \\
        total   & 253,836 & 455,877 & 2,794 & 234 & 4,397 & 112 & 10 & 47.49 & 78 & 2 & 31.08 \\
        \bottomrule
        \end{tabular}
    }
}
%\vspace{-0.1in}
\end{table*}

\begin{table*}[t]
\caption{The detailed statistics of GDELT-TE.}
\vspace{-0.1in}
\label{tab:detailed_stats_gdelt}
\centering
\setlength{\tabcolsep}{1mm}{
    \resizebox{0.9\textwidth}{!}{
        \begin{tabular}{l c c c c c ccc ccc}
        \toprule
        \multirow{2.4}{*}{subset} & \multirow{2.4}{*}{\#docs} & \multirow{2.4}{*}{\shortstack{\#ttl atomic \\ events}} & \multirow{2.4}{*}{$|\mathcal{E}|$} & \multirow{2.4}{*}{$|\mathcal{R}|$} & \multirow{2.4}{*}{\#CEs} & \multicolumn{3}{c}{\#atomic events/CE} & \multicolumn{3}{c}{\#time span (days)} \\
        \cmidrule(lr){7-9} \cmidrule(lr){10-12} & & & & & & max & min & avr & max & min & avr \\
        \midrule
        train   & 101,487 & 441,120   & 1,546 & 233 & 3,561 & 306 & 10 & 123.88 & 78 & 2 & 29.82 \\
        val     & 14,867  & 66,785    & 1,127 & 207 & 500   & 306 & 10 & 133.57 & 78 & 2 & 34.55 \\ 
        test    & 13,302  & 65,433    & 1,122 & 204 & 474   & 306 & 10 & 138.04 & 78 & 2 & 34.85 \\
        outlier & 144,352 & 628,543   & 1,553 & 231 & -     & -   & -  & -      & -  & - & -     \\
        total   & 273,845 & 1,201,881 & 1,555 & 239 & 4,535 & 306 & 10 & 126.43 & 78 & 2 & 30.87 \\
        \bottomrule
        \end{tabular}
    }
}
% \vspace{0.1in}
\end{table*}

\begin{table*}[!t]
\centering
\caption{An examples of the EE prompt.}
\vspace{-0.1in}
\label{tab:example_prompt_ee}
\begin{tabular}{p{0.97\textwidth}}
    \toprule
    You are an assistant to perform structured event extraction from news articles with following rules: \\ \\
        
    \textbf{[Rules:]} 1. Extract each event in format: event actor 1; event relation; event actor 2. \\
    2. Only choose event relation from this relation candidate list: Make public statement, Make an appeal or request, Express intent to cooperate, Consult or meet, Engage in diplomatic cooperation, Engage in material cooperation, Provide aid, Yield or concede, Investigate, Demand or order, Verbally disapprove, Reject, Threaten, Engage in political dissent, Exhibit military or police power, Reduce relations, Coerce, Use unconventional violence including terrorist, Use conventional military force, Use unconventional mass force. \\
    3. Event actors are usually political actors, countries or international organizations. \\
    4. Only extract events that have happened or is happening, and not extract future events. \\ \\
        
    \textbf{[Example:]} For example, given the example article: \\
    Egypt committed to boosting economic cooperation with Lebanon (MENAFN- Daily News Egypt) Egypt is committed to enforcing economic cooperation with Lebanon, President Abdel Fattah Al-Sisi said during his meeting with Lebanese parliamentary speaker Nabih Berri. \\
    List all events by rules, the extraction result of the example is: \\
    Egypt; Express intent to cooperate; Lebanon | Egypt president Abdel Fattah Al-Sisi; Consult or meet; Lebanese parliamentary speaker Nabih Berri | Lebanese parliamentary speaker Nabih Berri; Consult or meet; Egypt president Abdel Fattah Al-Sisi \\ \\
        
    \textbf{[News Article:]} Now, given the query article: \\
    Sudan security forces kill two anti-coup protesters - medics KHARTOUM, Sudan - Sudanese security forces killed two protesters in Omdurman, twin city of the capital Khartoum, medics says, as thousands rallied against the military. The pro-democracy Doctors' Committee says one of the protesters was shot in the chest while the second suffered a "severe head wound. Today's deaths bring the total number of protesters killed in a violent crackdown since a military takeover in October to 56, while hundreds have been wounded. \\ \\
        
    \textbf{[Output:]} List all events by rules, the extraction result of the query article is: \\
    \bottomrule
\end{tabular}
\end{table*}

\subsubsection{Structured Event Extraction}~\label{subsubsec:EE}
\textbf{Event Extraction.} We use the Vicuna-13b~\footnote{\url{https://github.com/lm-sys/FastChat}} to extract events from news articles. To fit the model to a single GPU card with 24GB memory, we apply the 8bit quantization strategy. Since the total number of atomic event types is more than 200, we cannot input all of them into one prompt due to the input limitation of Vicuna. Fortunately, CAMEO has a three-layer hierarchical structure, thus enabling us to do the extraction hierarchically. Specifically, we first input the news article and the first level atomic event types, asking the Vicuna to extract all the first-level events. Then, we parse the first-level extraction results. For each valid first-level event, we input its affiliated second-level atomic event types as options to the Vicuna model, together with the original news article, thus obtaining the second-level extraction results. The same procedure applies to the third-level event extraction. In order to extract events from all the 586,691 news articles (even though half of them are removed after filtering, we need the EE results to do the filtering.), it takes 2282 GPU hours in total (less than two weeks with eight A5000 Nvidia GPUs), of which each extraction takes about 14 seconds. The cost and efficiency are totally acceptable for general academic research labs.

We also demonstrate one example~\footnote{Here is the \href{https://www.newarab.com/news/sudan-security-forces-kill-two-anti-coup-protesters-medics}{source url} of this example news article.} of our first-level prompt in Table~\ref{tab:example_prompt_ee}. Our prompt mainly consists of three parts: 1) the extraction rules and candidate event types, 2) one example for in-context learning, and 3) the target news article. From the above example prompt, we can see that the target news article only takes a small portion of the whole input, while the rules and examples are quite long. However, the rules and examples are indispensible, otherwise, the quality of EE could dramatically drop. Furthermore, the EE performance of Vicuna also deteriorates when the input keeps increasing. Therefore, we only take the title and first three paragraphs of each news article as input to do the EE, based on our empirical observation that the salient events are usually reported in the title and first paragraphs in a news article. 

\begin{table*}[!t]
\centering
\caption{An example of the entity linking prompt.}
\vspace{-0.1in}
\label{tab:example_prompt_entity_linking}
\begin{tabular}{p{0.97\textwidth}}
    \toprule
    \textit{[the entity list]} Based on the above entity list. Perform entity linking with the following rules: \\
    1. Only merge entities that EXACTLY refer to the same entity such as PERSON, ORGANIZATION, COUNTRY, etc. \\
    2. The output key should be the entity name after merging, value should be list of original entity names. \\
    3. For those entities that cannot be merged, just output original name: {[}original name{]} \\
    4. There may be some noises in the strings, such as 'U.S.' or '1. U.S.', these cases should be merged but you should not clean the original name. \\
    5. Output in JSON format. \\
    \bottomrule
\end{tabular}
\end{table*}

\textbf{Entity Linking.} Since we do not have a pre-defined entity set during EE, the extracted entities have free forms and multiple entities correspond to the same one. We then perform entity linking, which is also a typical step in previous TCE construction studies~\cite{theFuture,resin}, using the current SOTA LLM GPT-4. More importantly, the entity set before linking is relatively small with several thousands, thus the cost of using GPT-4 is marginal. We first apply a K-means clustering over all the original entities to group the entities into multiple groups. Then we input the entities of each cluster as one batch and ask the GPT-4 to perform entity linking. We share an example~\footnote{Here is the \href{https://www.dailynewsegypt.com/2016/04/12/egypt-committed-boosting-economic-cooperation-lebanon/}{source url} of this example news article.} of the prompt for entity linking in Table~\ref{tab:example_prompt_entity_linking}.

Before the entity linking, we have 6322 entities after the aforementioned filtering. Then we use K-means to cluster them into 32 groups and input each group of entities to GPT-4 to perform the entity linking. To assure the potential same entities have the chance to be input to GPT-4 in the same batch, we iteratively perform such clustering + entity linking for two rounds. The final entity set of MidEast-TE is 2794. We do not perform any entity linking to the GDELT-TE dataset since its entity set is pre-defined.

\begin{figure*}
    \centering
    \includegraphics[width = 0.98\linewidth]{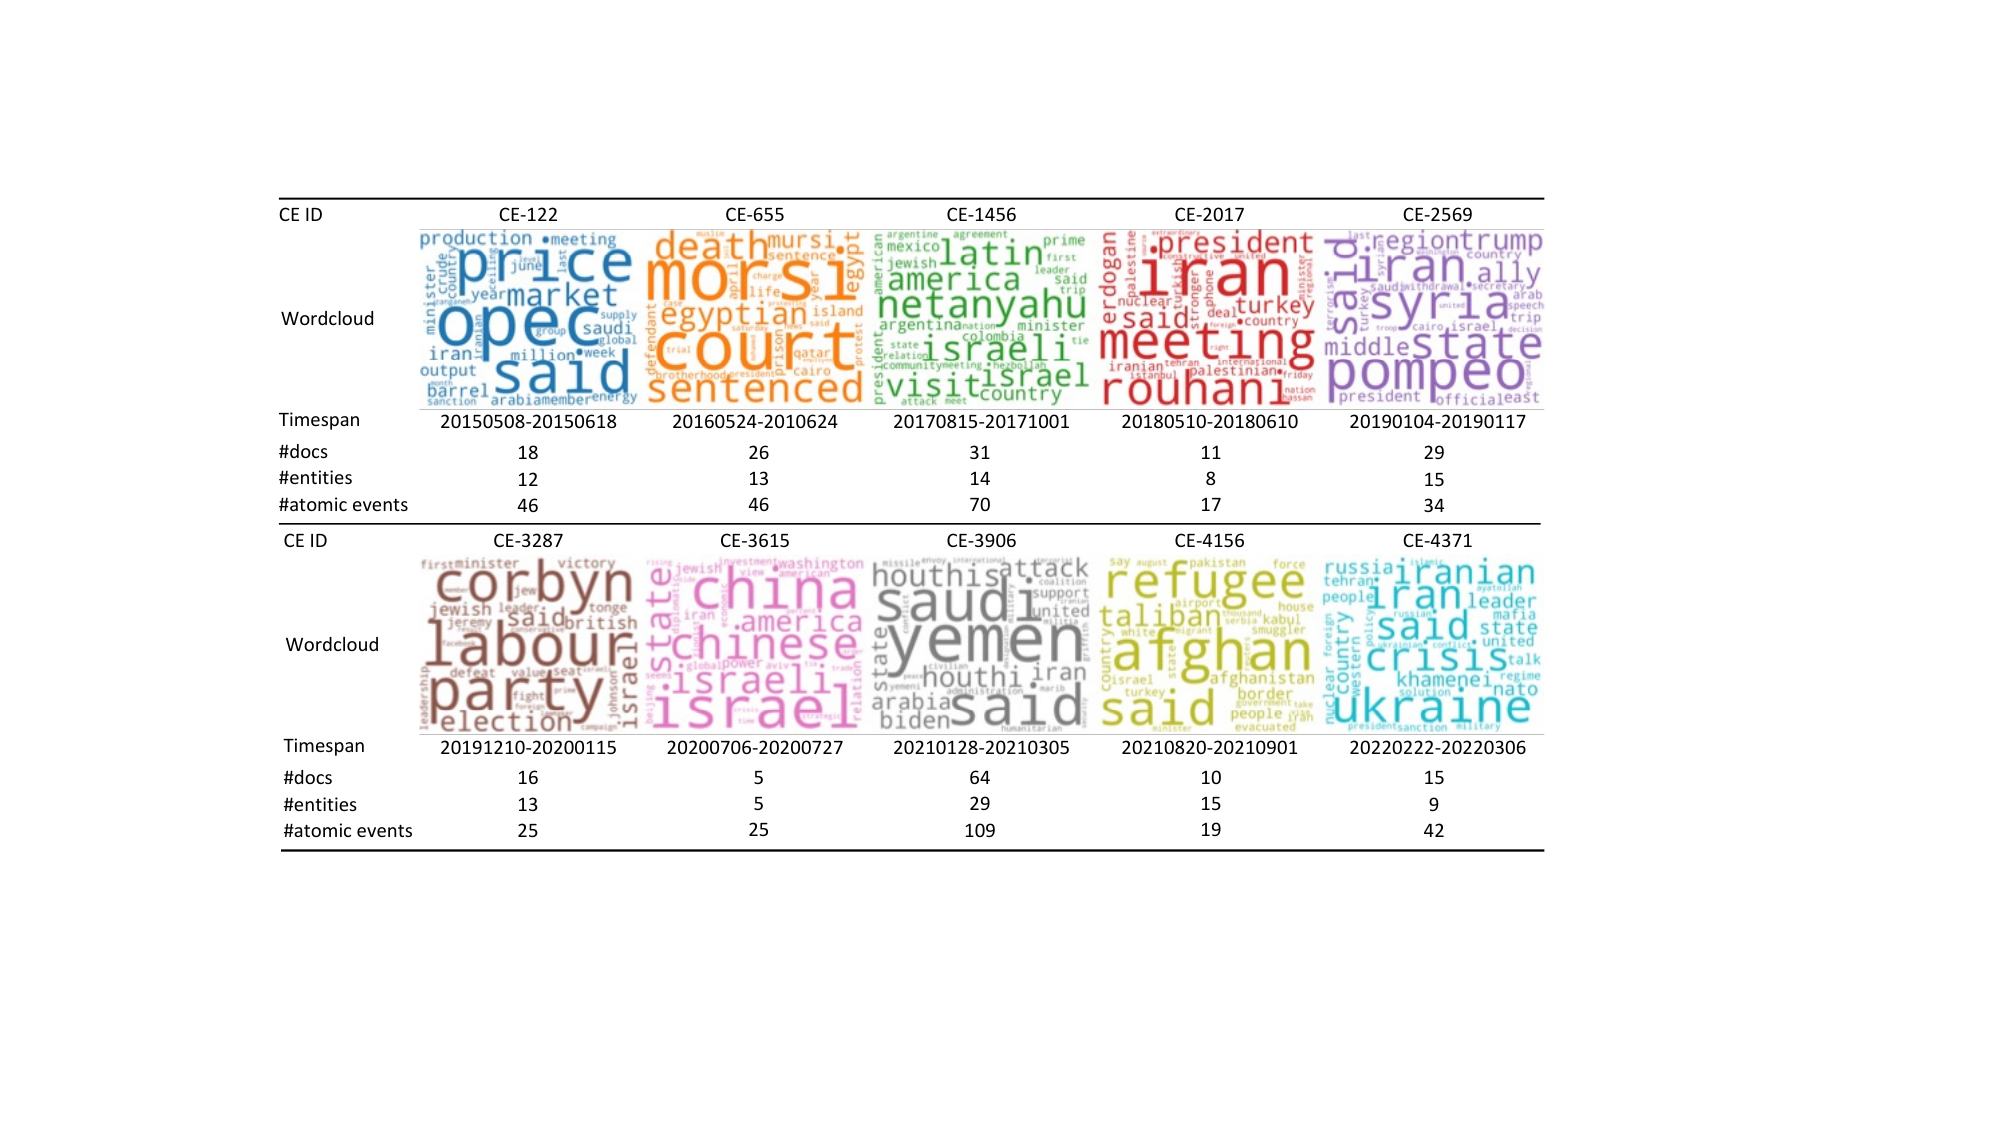}
    \vspace{-0.1in}
    \caption{Illustration of ten examples of CEs, each with its CE ID, wordcloud, timespan, number of involved news articles, entities, and atomic events.}
    %\vspace{-0.2in}
    \label{fig:example_CEs_wordcloud}
\end{figure*}

\begin{table*}[!t]
\caption{An example of the EE evaluation.}
\vspace{-0.1in}
\label{tab:example_prompt_ee_evaluation}
\begin{tabular}{p{0.97\textwidth}}
    \toprule
    You are an assistant to check the precision of event extraction from news articles. \\ \\
    \textbf{[Rules:]}
    1. Each extracted event is in format of "subject, relation, object". \\
    2. The check result is either True if the event is correct based on the article, otherwise False. \\
    3. Give a news article and a list of extracted events, you need to output the corresponding list of check results in json list format, for example: {[}True, False, True{]} \\ \\
    \textbf{[Article:]} Netanyahu Promises 'Crushing Blow' if Hezbollah Uses its 'Precision Rockets' Israeli PM Netanyahu has lashed out at recent comments made by Hezbollah leader Nasrallah, vowing to retaliate if Israel faces military action from the Lebanon-based Shia group. "If they confront us, they will suffer a crushing blow, the levels of which they cannot imagine," the PM said during an event at his office on Thursday. The statement came hours after Hassan Nasrallah, Secretary General of Hezbollah, threatened Israel with dire consequences should it wage a war on Lebanon, and announced that his group has acquired precision-guided missiles despite Israeli attempts to prevent it from attaining such weapons by striking targets in Syria. \\ \\ 
    \textbf{[Extracted Events:]} \\
    1. Israel; Refuse to comment; Hezbollah \\
    2. ISRAEL; Provide economic aid; IRAN \\
    3. HASSAN; Praise or endorse; TEHRAN \\
    4. LEBANON; Make public statement; ISRAEL \\
    5. ISRAEL; Praise or endorse; TEHRAN \\
    6. LEBANON; Make public statement; REUTERS \\ 
    7. HASSAN; Provide economic aid; IRAN \\
    8. LEBANON; Engage in symbolic act; ISRAEL \\
    9. ISRAELI; Criticize or denounce; HASSAN \\
    10. ISRAELI; Threaten with military force; LEBANON \\
    11. LEBANON; Praise or endorse; IRAN \\
    12. Hezbollah; Refuse to comment; Israel \\
    13. ISRAEL; Threaten with military force; LEBANON \\
    14. LEBANON; Engage in symbolic act; HASSAN \\ \\
    \textbf{[Results:]} Check result list: \\
    \bottomrule
\end{tabular}
\end{table*}

\subsubsection{Evaluation of the Datasets.} We specifically evaluate the three main steps of the dataset construction process, including clustering, event extraction, and entity linking. For the clustering, we sample some of them and plot their word clouds using tf-idf scores. The examples in Figure~\ref{fig:example_CEs_wordcloud} show that the clusters are distinct with each other, and each of the cluster focus on specific complex event. For the event extraction, we adopt more powerful commercial LLMs, \ie gpt-3.5 (which is more efficient and cheap compared with the most powerful GPT-4), to evaluate the extraction precision of both MidEast-TE and the GDELT-TE (the original EE system of GDELT). We sample 100 news articles from the entire datasets and input them as well as the extracted events into the prompt, then we ask the LLMs whether the extraction results are correct or wrong. The results show that the precision of MidEast-TE is 0.432 and the precision of GDELT-TE is 0.425. Overall speaking, the extraction performances of both LLMs and GDELT are still quite low. Nevertheless, our LLM-based EE is slightly better than the original GDELT. The open sourced Vicuna-13b verifies that it is possible to be used as a zero-shot EE model. In the future, we believe the performance of EE will be largely improved when more efficient and powerful LLMs are developed. For the entity linking, since the remaining entity set is small (2794), we manually check and fix the entity linking results, ensuring the linking result is correct.

We demonstrate an example~\footnote{Here is the \href{https://sputnikglobe.com/20180921/netanyahu-hezbollah-precision-rockets-1068220154.html}{source url} of this example news article.} of the gpt-3.5 prompt we used for EE evaluation in Table~\ref{tab:example_prompt_ee_evaluation}.

\subsection{Implementation Details} \label{app:subsec:exp_settings}
We implement all the static methods by ourselves. In terms of RE-NET, RE-GCN, and HisMatch, we reuse their officially released code and use the global context graph. We re-implement CMF by ourselves according to the original paper, and the textual embedding is extracted using the RoBERTa model fine-tuned by SimCSE. For all the baseline and our methods, only the atomic events within CEs are used as training samples and predicted during testing. For the outlier atomic events, they are just used as part of the input graph. To be fair, for all the methods, set the embedding dimensionality $d=200$, apply cross-entropy loss, grid search learning rate from $\{10^{-2}, 10^{-3}, 10^{-4}\}$ and weight decay from $\{10^{-4}, 10^{-5}, 10^{-6}, 10^{-7}\}$. We search the historical length $D$ from $\{1,3,5,7,10,14\}$ for all the TKG methods. The number of propagation layers of all the graph-based methods is grid searched from $\{1,2,3\}$. We use Adam~\cite{Adam} optimizer and Xavier~\cite{Xavier} initialization for all the methods.
